# Supplementary material for: Strategyproof Decision-Making in Panel Data Settings and Beyond
Source: arXiv:2211.14236 source file (2023-12-21)
Supplement: Supplementary file 4 [file model_proofs.tex]

\section{Proofs from Section~\ref{sec:setting}}
\begin{lemma}[Reward Reformulation]\label{prop:reward-app}
If $\sum_{t=T_0+1}^T \omega_t \cdot \pv{\vu}{d}_t \in \mathrm{span}(\{\pv{\vu}{0}_1, \ldots, \pv{\vu}{0}_{T_0} \})$, then $r_i^{(d)}$ can be written as
$r_i^{(d)} = \langle \pv{\vbeta}{d}, \vy_{i,pre} \rangle$,
for some $\pv{\vbeta}{d} \in \mathbb{R}^{T_0}$.
\end{lemma}
\begin{proof}
    From~\Cref{ass:lfm} and~\Cref{def:reward},
    \begin{equation*}
    \begin{aligned}
        r_i^{(d)} = \left \langle \sum_{t = T_0 + 1}^T \omega_t \cdot \vu_t^{(d)}, \mathbf{v}_i \right \rangle.
    \end{aligned}
    \end{equation*}
    Applying $\sum_{t=T_0+1}^T \omega_t \cdot \pv{\vu}{d}_t \in \mathrm{span}(\{\pv{\vu}{0}_1, \ldots, \pv{\vu}{0}_{T_0} \})$, 
    \begin{equation*}
    \begin{aligned}
        r_i^{(d)} = \left \langle \sum_{t = 1}^{T_0} \pv{\beta}{d}_t \cdot \vu_t^{(0)}, \mathbf{v}_i \right \rangle
    \end{aligned}
    \end{equation*}
    for some $\pv{\vbeta}{d} = [\pv{\beta}{d}_1, \ldots, \pv{\beta}{d}_{T_0}]^\top \in \mathbb{R}^{T_0}$.
\end{proof}
